# Supplementary material for: Enumerating consistent subgraphs of directed acyclic graphs: an insight into biomedical ontologies
Source: arXiv:1712.09679 source file (2017-12-27)
Supplement: Supplementary file 1 [file supplementary.pdf]

# Supplementary Materials
# Enumerating consistent subgraphs of directed acyclic graphs: an insight into biomedical ontologies

Yisu Peng[*], Yuxiang Jiang[*], and Predrag Radivojac

Department of Computer Science, Indiana University, Bloomington, Indiana, U.S.A.

This document contains supplementary text, algorithms, and detailed results related to the main manuscript.

## S1 Implementation Details

### S1.1 Handling Large Integers

The GNU Multiple Precision Arithmetic Library, available at `https://gmplib.org/`, was used to operate with large integers.

### S1.2 Source Code

The `cdag` algorithm is implemented in C++ and is freely available from GitHub, at the following location: `https://github.com/shawn-peng/counting-consistent-sub-DAG`.

## S2 Simulated directed acyclic graphs

We used Algorithm S1 to generate random directed acyclic graph in Section 5.1.

## S3 Empirical Verification of Correctness

We generated over 100,000 random graphs with a single root and the number of vertices less than or equal to 25 (Algorithm S1). The in-degrees of the vertices were generated according to a Poisson distribution whose parameter $\lambda$ was in turn sampled from a Gamma prior $\Gamma(2.0, 1.0)$. The parameter $\lambda$ was kept constant in each individual graph and then generated anew for the next graph.

A brute-force program was used to verify the correctness of our algorithm. This program simply generates all vertex-induced subgraphs of the input graph and then checks for their consistency.

[*]Contributed equally to this work.

**Algorithm S1:** Generating a random directed acyclic graph.

**Input :** Desired number of vertices $N_v$ of the DAG, Gamma shape parameters $(\alpha, \beta)$
**Output:** A directed acyclic graph $\mathcal{O}$

**Function** randdag($\mathcal{O}$)
  $\lambda \sim \Gamma(\alpha, \beta)$
  add vertex(1) to $\mathcal{O}$ as root
  **for** $i = 2$ *to* $N_v$ **do**
    $X \sim \text{Pois}(\lambda)$
    $n_p \leftarrow \min(X, |\mathcal{O}.V|)$
    add vertex($i$) to $\mathcal{O}$
    select random $n_p$ vertices from $\mathcal{O}.V$
    set these $n_p$ vertices to be parents of vertex($i$)
  **end**
**end**

# S4 Proof for the Minimum Bound Pivot Selection

The following proposition is used for the "minimum bound" pivot selection strategy in the acceleration of the algorithm.

**Proposition S4.1.** *Given an ontology $\mathcal{O}$, let $n$, $e$, $r$ be the number of its vertices, edges and roots, respectively. The quantity $U = e - n + r$ is an upper-bound of the number of multi-parent vertices ($m$) in $\mathcal{O}$.*

*Proof.* We prove this proposition by induction on the number of vertices. Since an ontology is a DAG, there exists a topological order of all vertices, say $v_1, v_2, \ldots, v_n$. We consider a graph reconstruction by adding back vertices along with its incoming edges in this order.

Staring from an empty graph, we have both $m$ and $U$ being equal to 0, so the upper-bound holds. Suppose now that this bound holds for all graphs of size $n = k$; i.e., $U^{(k)} \geq m^{(k)}$. Add the next vertex $v_{k+1}$ whose incoming degree is $d$.

If $d \geq 1$, we have $e^{(k+1)} = e^{(k)} + d$, $n^{(k+1)} = n^{(k)} + 1$ and $r^{(k+1)} = r^{(k)}$, hence

$$\begin{aligned} U^{(k+1)} &= U^{(k)} + (d-1) \\ &\geq m^{(k)} + (d-1) \\ &\geq m^{(k)} + \min(d-1, 1) \\ &= m^{(k+1)}. \end{aligned}$$

Otherwise, $d = 0$; i.e., the next vertex being added is a root, in which case $e^{(k+1)} = e^{(k)}$, $n^{(k+1)} = n^{(k)} + 1$ and $r^{(k+1)} = r^{(k+1)} + 1$; hence,

$$U^{(k+1)} = U^{(k)} \geq m^{(k)} = m^{(k+1)}.$$

Therefore, this upper-bound holds for both cases, and by induction, the proposition holds. □

# S5 Additional Algorithms

Here we show the additional algorithms that are called in the advanced algorithm in the main paper: (i) the extended algorithm on trees (ii) the algorithm that identifies all branching vertices

and (iii) the flow algorithm which is used in both branching vertex detection and one of the pivot strategies.

**Algorithm S2:** The generalized version of `ctree` for trees.

**Input :** A tree $\mathcal{T}_r$, rooted at $r$.
**Output:** The number of consistent subgraphs in $\mathcal{T}_r$.

**Function** `ctree`$^*(\mathcal{T}_r)$
  **if** $\mathcal{T}_r$ *is empty* **then**
    **return** 1;
  **else**
    **return** $\varphi(r) + \prod_{u \in \mathcal{C}(r)}$ `ctree`$^*(\mathcal{T}_u)$ ;   `// compatible with pruning, reversing`
    ;
  **end**
**end**

**Algorithm S3:** Branching vertex detection.

**Input :** A directed acyclic graph $\mathcal{O}$
**Output:** The branching vertices in $\mathcal{O}$ in a reversed topological order.

**Function** `branching_vertices`$(\mathcal{O})$
  `flow`$(\mathcal{O})$;
  **foreach** $v$ *in* $\mathcal{O}$ *in a reversed topological order* **do**
    **if** $v.flow = |\mathcal{D}^+(v)|$ **then**
      `append`$(list, v)$;
    **end**
  **end**
  **return** $list$;
**end**

# S6 Results on Biomedical Ontologies

This section provides more precise counts of consistent subgraphs in four biomedical ontologies, as discussed in Section 5.2 of the main paper and visualized in Figure 4. Table S1 provides counts that were completed before submitting this manuscript. The exact counts are available upon request.

**Algorithm S4:** Propagate flows in a DAG.

**Input :** A directed acyclic graph $\mathcal{O}$

**Output:** $\mathcal{O}$ with flow value saved to each vertex.

**Function** `flow`($\mathcal{O}$)

  **foreach** *$v$ in $\mathcal{O}$ in a reversed topological order* **do**

    $v.flow \leftarrow 1 + \sum_{u \in \mathcal{C}(v)} (u.flow / |\mathcal{P}(u)|)$

  **end**

  **return** $\mathcal{O}$;

**end**

Table S1: Number of consistent subgraphs in biomedical ontologies including vertices with up to a particular level. $n$: number of vertices, $e$: number of edges, $m$: number of multi-parent vertices, $\ell$: number of leaves.

| Ontology | level | $n$ | $e$ | $m$ | $\ell$ | count | lower bound | upper bound |
|---|---|---|---|---|---|---|---|---|
| MFO | 2 | 21 | 20 | 0 | 20 | 1.048e6 | 1.048e6 | 1.048e6 |
| | 3 | 156 | 155 | 0 | 143 | 5.465e43 | 1.115e43 | 5.465e43 |
| | 4 | 662 | 728 | 54 | 578 | 3.202e179 | 9.893e173 | 1.244e181 |
| | 5 | 2169 | 2460 | 247 | 1870 | 1.497e583 | 8.435e562 | 7.451e587 |
| | 6 | 6587 | 7403 | 722 | 5860 | 2.504e1812 | 1.086e1764 | 6.573e1827 |
| | 7 | 8394 | 9532 | 1014 | 7237 | 1.505e2256 | 3.582e2178 | 1.381e2279 |
| | 8 | 9415 | 10816 | 1226 | 7935 | - | 4.710e2388 | 1.077e2524 |
| | 9 | 9996 | 11621 | 1407 | 8306 | - | 2.265e2500 | 3.045e2659 |
| | 10 | 10300 | 12094 | 1536 | 8481 | - | 1.085e2553 | 9.609e2725 |
| | 11 | 10470 | 12430 | 1648 | 8573 | - | 5.372e2580 | 5.868e2763 |
| | 12 | 10641 | 12755 | 1755 | 8639 | - | 3.964e2600 | 2.209e2802 |
| | 13 | 10709 | 12861 | 1780 | 8672 | - | 3.405e2610 | 5.656e2816 |
| | 14 | 10762 | 12997 | 1828 | 8697 | - | 1.143e2618 | 2.554e2830 |
| | 15 | 10779 | 13025 | 1835 | 8703 | - | 7.312e2619 | 8.018e2833 |
| | 16 | 10788 | 13044 | 1843 | 8703 | - | 7.312e2619 | 4.021e2835 |
| | 17 | 10789 | 13046 | 1844 | 8703 | - | 7.312e2619 | 5.577e2835 |
| MFO$^u$ | 2 | 20 | 19 | 0 | 19 | 5.242e5 | 5.243e5 | 5.242e5 |
| | 3 | 143 | 142 | 0 | 130 | 6.724e39 | 1.361e39 | 6.724e39 |
| | 4 | 541 | 595 | 43 | 463 | 8.386e144 | 2.382e139 | 1.970e146 |
| | 5 | 1561 | 1789 | 188 | 1282 | 6.191e405 | 8.326e385 | 2.966e410 |
| | 6 | 3688 | 4299 | 524 | 3033 | 5.892e959 | 1.057e913 | 8.019e973 |
| | 7 | 4952 | 5811 | 751 | 3924 | 6.943e1257 | 1.745e1181 | 4.438e1278 |
| | 8 | 5704 | 6780 | 926 | 4403 | 2.387e1424 | 2.723e1325 | 1.672e1454 |
| | 9 | 6108 | 7360 | 1069 | 4619 | 1.239e1503 | 2.868e1390 | 6.152e1541 |
| | 10 | 6342 | 7709 | 1161 | 4740 | - | 7.624e1426 | 4.269e1591 |
| | 11 | 6474 | 7977 | 1253 | 4804 | - | 1.406e1446 | 1.493e1620 |
| | 12 | 6591 | 8200 | 1327 | 4842 | - | 3.866e1457 | 5.313e1645 |
| | 13 | 6634 | 8268 | 1344 | 4860 | - | 1.013e1463 | 4.432e1654 |
| | 14 | 6654 | 8320 | 1363 | 4870 | - | 1.038e1466 | 3.623e1659 |
| | 15 | 6661 | 8333 | 1367 | 4872 | - | 4.151e1466 | 7.937e1660 |
| | 16 | 6662 | 8334 | 1367 | 4872 | - | 4.151e1466 | 1.160e1661 |

| Ontology | level | $n$ | $e$ | $m$ | $\ell$ | count | lower bound | upper bound |
|---|---|---|---|---|---|---|---|---|
| BPO | 2 | 22 | 21 | 0 | 21 | 2.097e6 | 2.097e6 | 2.097e6 |
| | 3 | 123 | 147 | 25 | 101 | 2.376e31 | 2.535e30 | 1.311e32 |
| | 4 | 573 | 734 | 149 | 471 | 1.430e147 | 6.097e141 | 4.118e150 |
| | 5 | 1777 | 2631 | 672 | 1365 | - | 8.053e410 | 1.177e453 |
| | 6 | 4288 | 7182 | 2049 | 3057 | - | 1.773e920 | 1.616e1067 |
| | 7 | 8109 | 14783 | 4593 | 5198 | - | 5.674e1564 | 8.161e1961 |
| | 8 | 12719 | 24596 | 7966 | 7449 | - | 2.357e2242 | 4.714e3004 |
| | 9 | 17243 | 34704 | 11414 | 9397 | - | 6.010e2828 | 1.309e4015 |
| | 10 | 21445 | 44378 | 14816 | 11036 | - | 1.469e3322 | 1.247e4938 |
| | 11 | 24683 | 51711 | 17443 | 12102 | - | 1.161e3643 | 3.029e5637 |
| | 12 | 26944 | 56834 | 19280 | 12780 | - | 1.457e3847 | 3.641e6118 |
| | 13 | 28424 | 60105 | 20489 | 13231 | - | 8.470e3982 | 1.518e6433 |
| | 14 | 29134 | 61702 | 21071 | 13401 | - | 1.268e4034 | 2.585e6577 |
| | 15 | 29402 | 62314 | 21294 | 13439 | - | 3.484e4045 | 2.794e6630 |
| | 16 | 29509 | 62551 | 21377 | 13465 | - | 2.338e4053 | 9.061e6652 |
| | 17 | 29551 | 62648 | 21410 | 13477 | - | 9.577e4056 | 1.750e6661 |
| | 18 | 29572 | 62697 | 21431 | 13485 | - | 2.452e4059 | 5.407e6665 |
| | 19 | 29575 | 62700 | 21431 | 13487 | - | 9.807e4059 | 2.433e6666 |
| BPO$^u$ | 2 | 22 | 21 | 0 | 21 | 2.097e6 | 2.097e6 | 2.097e6 |
| | 3 | 114 | 137 | 24 | 92 | 2.714e29 | 4.952e27 | 2.714e29 |
| | 4 | 489 | 626 | 128 | 398 | 7.082e127 | 6.456e119 | 7.082e127 |
| | 5 | 1471 | 2219 | 585 | 1106 | - | 8.693e332 | 3.142e372 |
| | 6 | 3419 | 5776 | 1667 | 2353 | - | 2.107e708 | 6.968e841 |
| | 7 | 6267 | 11369 | 3539 | 3851 | - | 1.847e1159 | 1.062e1503 |
| | 8 | 9649 | 18501 | 5980 | 5359 | - | 1.659e1613 | 1.410e2257 |
| | 9 | 12935 | 25726 | 8461 | 6622 | - | 2.634e1993 | 8.698e2980 |
| | 10 | 15775 | 32228 | 10762 | 7518 | - | 1.392e2263 | 1.322e3589 |
| | 11 | 17932 | 37166 | 12525 | 8039 | - | 9.553e2419 | 2.283e4043 |
| | 12 | 19481 | 40657 | 13745 | 8405 | - | 1.436e2530 | 3.209e4367 |
| | 13 | 20472 | 42852 | 14565 | 8588 | - | 1.760e2585 | 1.618e4571 |
| | 14 | 20918 | 43853 | 14923 | 8639 | - | 3.964e2600 | 2.116e4658 |
| | 15 | 21077 | 44218 | 15053 | 8641 | - | 1.586e2601 | 4.939e4688 |
| | 16 | 21128 | 44336 | 15094 | 8640 | - | 7.928e2600 | 1.059e4698 |
| | 17 | 21148 | 44385 | 15111 | 8639 | - | 3.964e2600 | 3.202e4701 |
| | 18 | 21154 | 44402 | 15117 | 8641 | - | 1.586e2601 | 6.313e4702 |

| Ontology | level | $n$ | $e$ | $m$ | $\ell$ | count | lower bound | upper bound |
|---|---|---|---|---|---|---|---|---|
| CCO | 2 | 16 | 15 | 0 | 15 | 32769 | 32768 | 32769 |
| | 3 | 78 | 84 | 7 | 67 | 8.155e20 | 1.476e20 | 8.155e20 |
| | 4 | 351 | 413 | 52 | 301 | 4.895e94 | 4.074e90 | 3.441e95 |
| | 5 | 623 | 840 | 166 | 476 | 2.249e156 | 1.951e143 | 3.113e162 |
| | 6 | 953 | 1416 | 346 | 713 | 2.127e233 | 4.309e214 | 1.387e245 |
| | 7 | 1225 | 1881 | 470 | 880 | 3.543e291 | 8.061e264 | 9.098e310 |
| | 8 | 1737 | 2765 | 742 | 1301 | - | 4.365e391 | 1.110e451 |
| | 9 | 2185 | 3584 | 969 | 1600 | - | 4.446e481 | 4.844e565 |
| | 10 | 2619 | 4534 | 1292 | 1899 | - | 4.529e571 | 2.657e680 |
| | 11 | 3051 | 5482 | 1578 | 2164 | - | 2.685e651 | 5.198e786 |
| | 12 | 3491 | 6425 | 1887 | 2400 | - | 2.965e722 | 2.320e894 |
| | 13 | 3780 | 7105 | 2119 | 2540 | - | 4.132e764 | 3.286e962 |
| | 14 | 3964 | 7533 | 2255 | 2630 | - | 5.116e791 | 7.860e1006 |
| | 15 | 4061 | 7751 | 2321 | 2668 | - | 1.406e803 | 9.184e1029 |
| | 16 | 4082 | 7798 | 2336 | 2672 | - | 2.250e804 | 3.675e1034 |
| | 17 | 4084 | 7801 | 2337 | 2672 | - | 2.250e804 | 1.102e1035 |
| | 18 | 4085 | 7802 | 2337 | 2672 | - | 2.250e804 | 1.469e1035 |
| $CCO^u$ | 2 | 14 | 13 | 0 | 13 | 8193 | 8192 | 8193 |
| | 3 | 66 | 72 | 7 | 55 | 2.116e17 | 3.603e16 | 2.116e17 |
| | 4 | 269 | 316 | 38 | 228 | 5.486e71 | 4.314e68 | 2.721e72 |
| | 5 | 455 | 619 | 124 | 339 | 1.287e112 | 1.120e102 | 1.639e117 |
| | 6 | 675 | 1023 | 255 | 481 | 5.816e160 | 6.243e144 | 6.137e170 |
| | 7 | 864 | 1361 | 352 | 585 | 4.194e198 | 1.266e176 | 2.439e215 |
| | 8 | 1159 | 1945 | 558 | 794 | 7.022e266 | 1.042e239 | 4.178e291 |
| | 9 | 1441 | 2479 | 711 | 961 | - | 1.949e289 | 5.107e360 |
| | 10 | 1761 | 3176 | 954 | 1181 | - | 3.284e355 | 3.304e444 |
| | 11 | 2080 | 3886 | 1162 | 1357 | - | 3.146e408 | 7.276e521 |
| | 12 | 2376 | 4521 | 1372 | 1504 | - | 5.612e452 | 3.908e593 |
| | 13 | 2565 | 4966 | 1519 | 1591 | - | 8.684e478 | 3.450e637 |
| | 14 | 2695 | 5270 | 1613 | 1656 | - | 3.204e498 | 6.089e669 |
| | 15 | 2765 | 5432 | 1662 | 1682 | - | 2.150e506 | 7.189e686 |
| | 16 | 2775 | 5455 | 1668 | 1682 | - | 2.150e506 | 2.361e689 |
| | 17 | 2776 | 5456 | 1668 | 1682 | - | 2.150e506 | 3.541e689 |
| | 18 | 2777 | 5457 | 1668 | 1682 | - | 2.150e506 | 4.722e689 |

| Ontology | level | $n$ | $e$ | $m$ | $\ell$ | count | lower bound | upper bound |
|---|---|---|---|---|---|---|---|---|
| HPO | 2 | 6 | 5 | 0 | 5 | 33 | 32 | 33 |
| | 3 | 59 | 58 | 0 | 53 | 1.374e16 | 9.007e15 | 1.374e16 |
| | 4 | 285 | 288 | 4 | 238 | 3.946e73 | 4.417e71 | 4.199e73 |
| | 5 | 867 | 925 | 59 | 698 | 5.195e218 | 1.315e210 | 3.386e219 |
| | 6 | 2135 | 2340 | 199 | 1635 | - | 1.528e492 | 7.485e526 |
| | 7 | 4162 | 4695 | 508 | 3057 | - | 1.773e920 | 1.126e1003 |
| | 8 | 6375 | 7330 | 891 | 4514 | - | 7.079e1358 | 9.364e1506 |
| | 9 | 8307 | 9679 | 1270 | 5777 | - | 1.123e1739 | 1.740e1946 |
| | 10 | 9733 | 11489 | 1616 | 6653 | - | 5.657e2002 | 2.414e2264 |
| | 11 | 10700 | 12841 | 1958 | 7244 | - | 4.584e2180 | 2.020e2481 |
| | 12 | 11271 | 13892 | 2311 | 7508 | - | 1.359e2260 | 2.226e2605 |
| | 13 | 11709 | 14841 | 2641 | 7712 | - | 3.494e2321 | 1.920e2705 |
| | 14 | 12121 | 15862 | 3035 | 7872 | - | 5.107e2369 | 4.017e2806 |
| | 15 | 12149 | 15920 | 3054 | 7888 | - | 3.347e2374 | 1.085e2813 |
| | 16 | 12167 | 15974 | 3072 | 7891 | - | 2.677e2375 | 8.845e2817 |
| HPO$^u$ | 2 | 5 | 4 | 0 | 4 | 17 | 16 | 17 |
| | 3 | 45 | 44 | 0 | 40 | 1.753e12 | 1.100e12 | 1.753e12 |
| | 4 | 206 | 209 | 4 | 166 | 1.005e52 | 9.354e49 | 1.134e52 |
| | 5 | 606 | 656 | 51 | 463 | 2.224e147 | 2.382e139 | 1.227e148 |
| | 6 | 1481 | 1649 | 164 | 1062 | - | 4.941e319 | 5.988e353 |
| | 7 | 2785 | 3203 | 402 | 1871 | - | 1.687e563 | 1.123e647 |
| | 8 | 4097 | 4824 | 680 | 2625 | - | 1.599e790 | 3.328e930 |
| | 9 | 5213 | 6239 | 953 | 3241 | - | 4.347e975 | 1.581e1169 |
| | 10 | 6026 | 7328 | 1200 | 3653 | - | 4.598e1099 | 1.882e1338 |
| | 11 | 6470 | 7956 | 1357 | 3839 | - | 4.510e1155 | 3.712e1427 |
| | 12 | 6667 | 8289 | 1470 | 3884 | - | 1.587e1169 | 2.640e1466 |
| | 13 | 6745 | 8441 | 1518 | 3892 | - | 4.062e1171 | 8.671e1480 |
| | 14 | 6777 | 8524 | 1546 | 3874 | - | 1.550e1166 | 5.623e1486 |
| | 15 | 6783 | 8538 | 1552 | 3875 | - | 3.099e1166 | 7.346e1487 |
| | 16 | 6785 | 8544 | 1554 | 3873 | - | 7.748e1165 | 2.145e1488 |
